# Supplementary material for: Jetting with gels: Soft microgel networks stabilize and extend nozzle-free water jets
Source: arXiv:2508.21147 source file (2025-08-28)
Supplement: Supplementary file 1 [file suppl.pdf]

# Supporting Information: Jetting with gels: Soft microgel networks stabilize and extend nozzle-free water jets

Atieh Razavi, Mehrzad Roudini, Andreas Winkler, Benno Liebchen, Regine von Klitzing, Suvendu Mandal,* and Amin Rahimzadeh*

E-mail: suvendu.mandal@pkm.tu-darmstadt.de; Amin.rahimzadeh@pkm.tu-darmstadt.de

## S1 Overview of the jetting phenomenon.

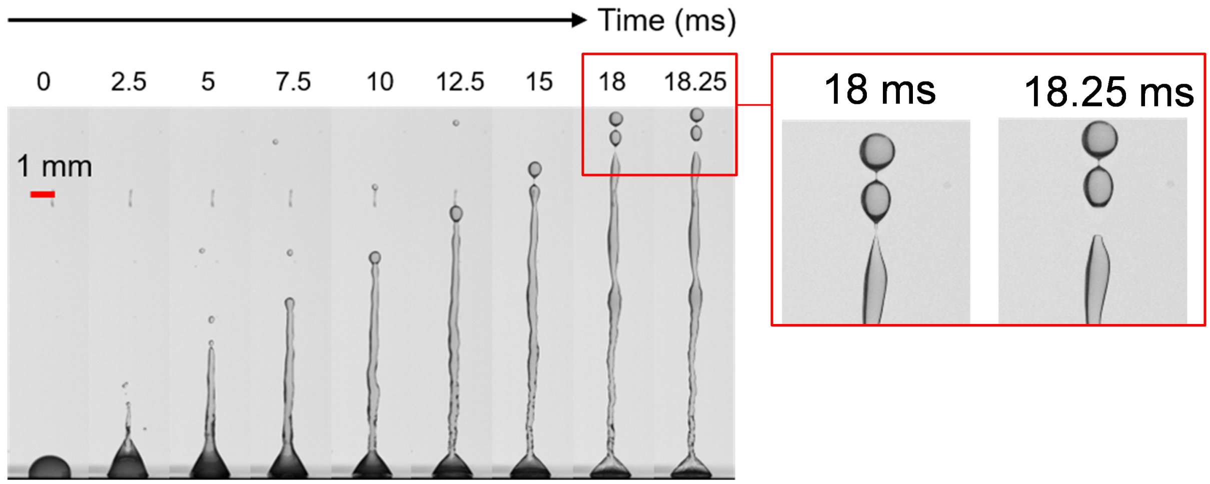


Figure S1: Jetting and break-up of a 1 wt% aqueous droplet containing microgels with 1 mol% cross-linker (MG1).

# S2 Surface tension of microgel dispersions

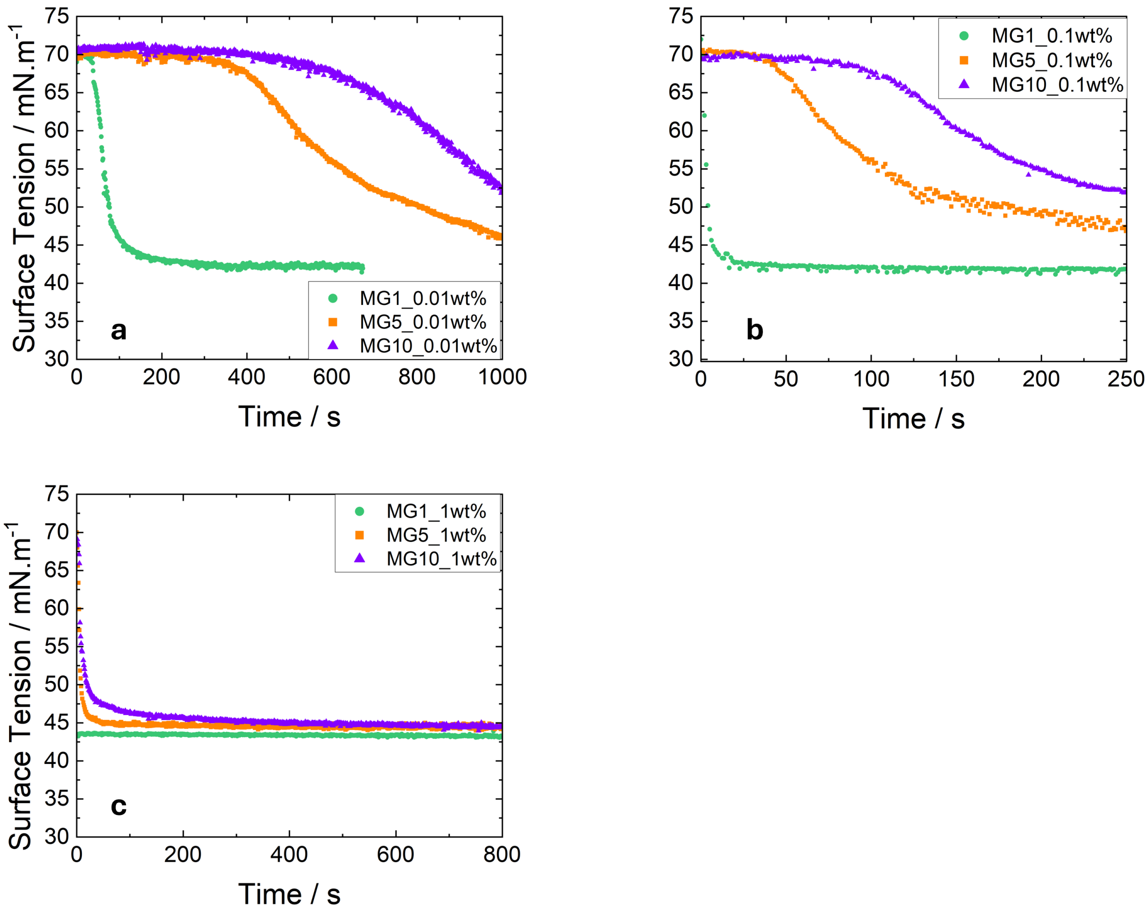


Figure S2: Surface tension of PNIPAM dispersions at different cross-linker content (i.e., stiffness) and various concentrations of a) 0.01 wt%, b) 0.1 wt%, and c) 1 wt%. The time scale varies due to different kinetics at various concentrations. Jetting occurs at around 20 ms.

# S3 Viscosity of microgel dispersions

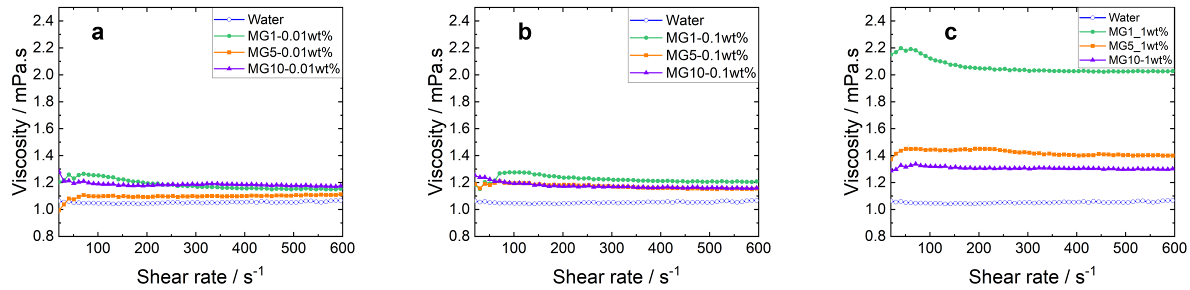


Figure S3: Shear viscosity of PNIPAM dispersions at different cross-linker content (i.e., stiffness) and various concentrations of a) 0.01 wt%, b) 0.1 wt%, and c) 1 wt% concentration.

# S4 Hydrodynamic radius at different temperatures

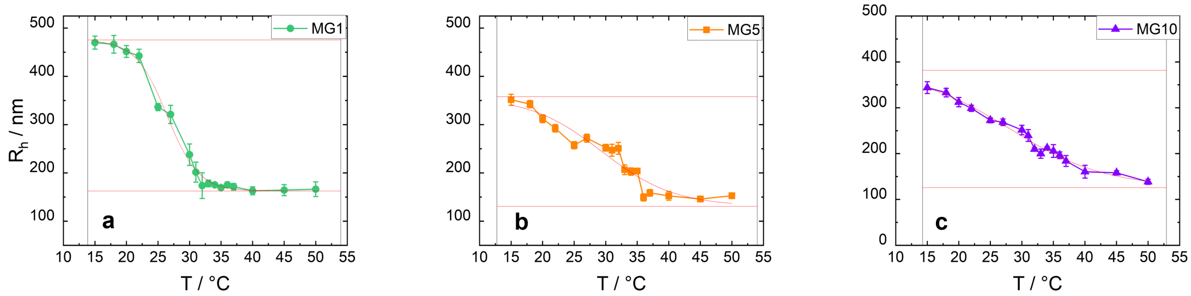


Figure S4: Hydrodynamic radius of PNIPAM microgels at different cross-linker contents of a) MG 1: 1 mol%, b) MG 5: 5 mol% and c) MG 10: 10 mol% cross-linker.
